# Supplementary material for: Data Augmentation for Continual RL via Adversarial Gradient Episodic Memory
Source: arXiv:2408.13452 source file (2024-10-16)
Supplement: Supplementary file 1 [file appendix.tex]

%%%%%%%%%%%%%%%%%%%%%%%%%%%%%%%%%%%%%%%%%%%%%%%%%%%%%%%%%%%%%%%%%%%%%%%%%%%%%%%
%%%%%%%%%%%%%%%%%%%%%%%%%%%%%%%%%%%%%%%%%%%%%%%%%%%%%%%%%%%%%%%%%%%%%%%%%%%%%%%
% APPENDIX
%%%%%%%%%%%%%%%%%%%%%%%%%%%%%%%%%%%%%%%%%%%%%%%%%%%%%%%%%%%%%%%%%%%%%%%%%%%%%%%
%%%%%%%%%%%%%%%%%%%%%%%%%%%%%%%%%%%%%%%%%%%%%%%%%%%%%%%%%%%%%%%%%%%%%%%%%%%%%%%
\newpage
\appendix
\onecolumn
\section{More details about Methods}

\begin{figure}[htb] 
% \begin{center}
\centerline{\includegraphics[width=0.6 \columnwidth]{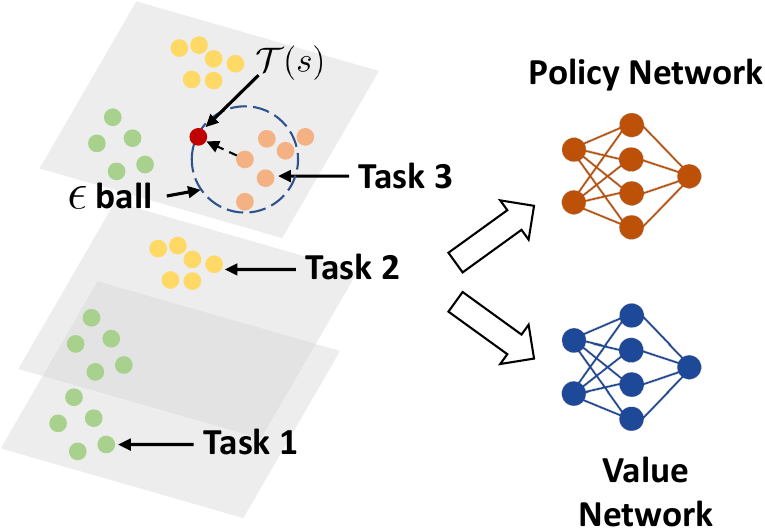}}
\caption{A conception illustration of data augmentation for continual RL among three tasks. The data augmentation  generates more diverse data samples during each task, which will be used to update the policy and value network of continual RL agent. 
% Initially, in task 1, the well-trained boundary could classify clearly. From task 1 to task 2, the boundary changed to fit task 2 correctly, while task 1 became harder to classify. Based on Adversarial Augmentation, the boundary could mitigate the wrong classification. The red arrow (corresponds to the adversarial term) generates adversarial example, and drives the boundary towards previous task data.
}
\label{figure:DA_overview}
% \vskip -0.2in
\end{figure}

\begin{figure}[htb] 
% \begin{center}
\centerline{\includegraphics[width=0.8 \columnwidth]{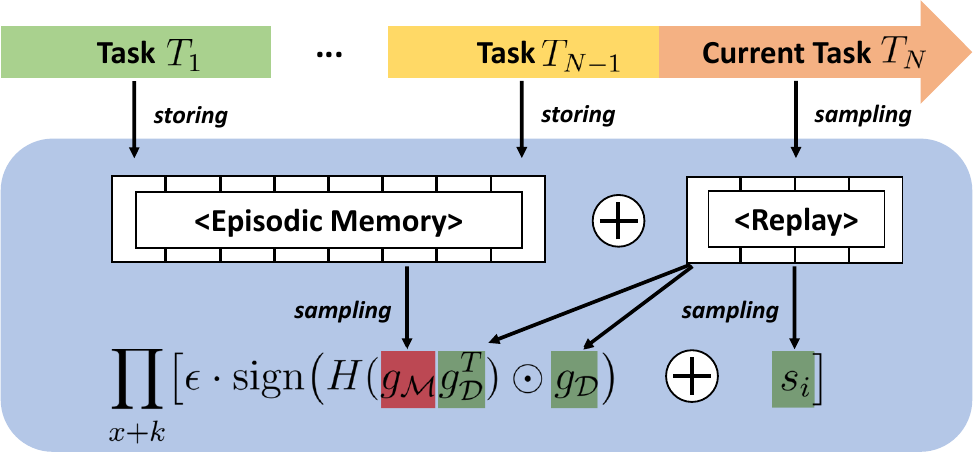}}
\caption{Process for Adv-GEM data generation. For each previous task, we store samples in the episodic memory $\mathcal{M}$. While we optimize the current task, we sample data from the replay buffer $\mathcal{D}$. We generate the adversarial examples by embedding the gradient episodic memory, where $H$ is the Heaviside step function, $g_{\mathcal{D}}$ is the gradient of the policy network at the current task, $g_{\mathcal{D}} = \nabla_{s_i \sim \mathcal{D}}\mathcal{L}_{\pi_{\theta}}(s_i)$, and $g_{\mathcal{M}}$ is the gradient of the policy network at the previous tasks, $g_{\mathcal{M}} = \nabla_{s_i \sim \mathcal{M}}\mathcal{L}_{\pi_{\theta}}(s_i)$.}
\label{figure-adversarialDA}
% \end{center}
\end{figure}

\begin{algorithm}[H] 
    \caption{Adv-GEM Augmentation}
    \label{alg_1}
\input{content/alg_adv_gem.tex}
\end{algorithm}
\section{Extended Related Work}
\subsection{Gradient Episodic Memory} \label{section:Gradient Episodic Memory}
% \citep{lopez2017gradient,chaudhry2018efficient,guo2020improved}

There are two well-used gradient-based episodic memory methods to mitigate catastrophic forgetting in CL,  GEM \citep{lopez2017gradient} and A-GEM \citep{chaudhry2018efficient}. Both methods require storing an episodic memory $M_k$ for each task $k$.

GEM \citep{lopez2017gradient} minimizes the loss of the current task $t$, while ensuring that each loss of the previous task $k<t$ remained not increased. The objective function is formalized as below:
\begin{align}
&\mathrm{minimize}_{\theta} \; \ell(f_{\theta}, D_t), \\
&\mathrm{s.t.}\quad\ell(f_{\theta},M_k) \leq \ell (f_{\theta}^{t-1}, M_k), \quad \forall k<t, \nonumber
\end{align}
where $f_{\theta}^{t-1}$ is the trained network parameters after task $t-1$. 
% To prevent the increase of loss on each previous tasks $k$, GEM calculate the angle between the gradient $g$ of the current task and the gradients of each previous tasks $g_k$, while the angle is lager than $90^{\circ}$ with any of the $g_k$, GEM will project the gradient $g$ of current task within the L2 norm bound. 
The minimization problem of GEM is formalized by:
\begin{equation}
\mathrm{minimize}_{\tilde{g}} \quad \frac{1}{2}\lVert g - \tilde{g} \rVert_{2}^{2} \quad \mathrm{s.t.} \quad\langle \tilde{g},g_k \rangle \geq 0 \quad \forall k<t.
\end{equation}
A-GEM \citep{chaudhry2018efficient} replaces the loss of each \textit{individual} previous tasks with \textit{average} episodic memory loss.
% to ensure the performance of previous task does not increase after update.
\begin{align}
&\mathrm{minimize}_{\theta} \; \ell(f_{\theta}, D_t), \\
&\mathrm{s.t.}\,\ell(f_{\theta},M)\leq \ell(f_{\theta}^{t-1}, M)\; \mathrm{where} \, M=\cup_{k<t}M_k. \nonumber
\end{align}
Therefore, the optimization problem is simplified to:
\begin{equation} \label{eq_9}
\mathrm{minimize}_{\tilde{g}} \quad \frac{1}{2}\lVert g - \tilde{g} \rVert_{2}^{2}, \quad \mathrm{s.t.} \quad {\tilde{g}}^T g_{ref} \geq 0.
\end{equation}
where $g_{ref} = \nabla{\ell(f_{\theta}^{t-1}, M)}$ is calculated based on a random subset of all previous tasks. 

The constrained Eq. \ref{eq_9} can be optimized efficiently based on \citep{chaudhry2018efficient}. When gradient $g$ breaks the constrain, it will be projected as below:
\begin{equation}
\tilde{g} = g - \frac{g^Tg_{ref}}{g^T_{ref}g_{ref}}g_{ref}.
\end{equation}
The above Gradient-based Episodic Memory methods indicate that modifying the gradient according to previous tasks' gradient can promise the mitigation of forgetting. Actually, in our paper, we will adapt the gradient of the previous tasks as the guidance of adversarial attack. 

\subsection{Adversarial Attack} \label{section:adversarial-attack}
The existing literature on adversarial attack \citep{goodfellow2014explaining, madry2017towards, croce2020reliable} is quite close to this work, with the same idea to devise training processes to enhance the robustness of the model. As the first well-known work, the Fast Gradient Sign Method (FGSM) \citep{goodfellow2014explaining} generated imperceptible perturbations by calculating the first-order gradient within $\epsilon$-ball, also with several variations \citep{kurakin2016adversarial, tramer2017space}. Later, \citep{madry2017towards} proposed the Projected Gradient descent (PGD) and achieved significant adversary, which is a very powerful method not only in adversarial attack but also in adversarial training. Additionally, considering the unsupervised domain adaptation problem, \citep{9528987} investigated from adversarial attack perspective and tackle the divergence-agnostic adaptive learning problem, which has few similarities with our work.

To penalize the differences between  the original and the adversarial examples, adversarial training paradigm was developed, like \citep{sinha2017certifying, madry2017towards, heinze2017conditional}. \citep{sinha2017certifying} proposed a unified adversarial training architecture, by maximizing the worst-case data distribution while optimizing the model parameters with respect to the adversarial examples. Developed from it, \citep{10.5555/3327345.3327439} imposed the constraint in the semantic space, aiming to learn models that are resistant to out-of-distribution samples. 

The adversarial attack also has shown its effectiveness on RL. In \citep{huang2017adversarial}, they obtained the adversarial examples by directly using FGSM \citep{goodfellow2014explaining} to perturb each image at every time step for RL. 
Further, relying on the sequential decision-making property of RL, \citep{lin2017tactics} propose strategically-attack that attacks at critical moments will be more efficient, and enchanting-attack that maliciously lures an agent to a certain state.

Adversarial training \citep{madry2017towards} can be regarded as the combination of an \textit{inner maximization} problem and an \textit{outer minimization} problem. The outer minimization problem will optimize the model to be resistant to perturbations. Formally, this min-max  optimization problem can be written as 
\begin{equation}
\underset{\theta}{\mathrm{min}}\;{{\mathbb{E}}_{(x,y) \sim D}[\underset{||\delta||_p<\epsilon}{\mathrm{max}}(\mathcal{L}(\theta,x + \delta,y))]},
\end{equation}
where $\delta$ represents the perturbation distance within the radius $\epsilon$.

The inner maximization problem is to find the adversarial examples, where FGSM \citep{goodfellow2014explaining} and PGD \citep{madry2017towards} are two common methods.
FGSM \citep{goodfellow2014explaining} generates adversarial samples by the one-step update:
\begin{equation}
x_{adv} = x + \epsilon \, \mathrm{sgn}(\nabla_x{\mathcal{L}(\theta,x,y)}).
\end{equation}
While PGD \citep{madry2017towards} can be interpreted as a multiple-steps scheme for maximizing the loss function, the adversarial sample is obtained by:
\begin{equation}
x_{adv} = \prod_{x+k}(x + \epsilon \,  \mathrm{sgn}(\nabla_x{\mathcal{L}(\theta,x,y)}).
\end{equation}
This actually is the idea behind our adversarial augmentation, specifically applied in continual learning with memory-gradient embedded.

\newpage
\section{More details about Experiments}
\subsection{Implementation and Evaluation}
\textbf{Implementation detail.} 
To ensure the fairness of comparison, the SAC parameters and network architecture keep the same with Continual World \citep{wolczyk2021continual}. For the basic data augmentations, we set the parameters as below. We use a $\alpha$ and $\sigma$ of 1.0 in Uniform noise and Gaussian noise, respectively. In RAS, we choose $\alpha = 0.9$ and $\beta = 1.1$ to preserve the signs of the states. In mixup, we sample $\lambda$ from Beta distribution with the $\alpha = 0.4$ as in \citep{zhang2017mixup}. For Adv-AUG and Adv-GEM, the norm ball of the adversarial attack $\epsilon$ is set as $0.1$. And the iteration time $k$ is set as 1, since the high computation cost of PGD within RL training. Further, the memory buffer size $N_\mathcal{M}$ is set as $10\mathrm{k}$ in Adv-GEM. All reported results in MW4, are the average results from 5 seeds with 90\% confidence intervals. All of the results for CW10 are run for 3 seeds with 90\% confidence intervals.
% We set the augmentation start timesteps $S$ as 300k for each task, augmentation phase gap $\delta$ as 50k, augmentation probability $\lambda$ as 0.5.

\textbf{Evaluation Metrics.} \label{evaluation-metrics} Below we describe the metrics used to evaluate the continual RL methods studied in this paper. For each task, we train for $\Delta = 1M$ steps. Considering we have $N$ tasks in sequences, the total sample budget is $T = \Delta \cdot N$.  During the task step $[t \in [(i-1)\cdot\Delta,i\cdot\Delta]$, the $i$-th task is trained for one certain environment. Hereby, we report the average performance, forward transfer and catastrophic forgetting as below.    
\begin{itemize}[leftmargin=*]
\item \textbf{Average Performance.} The performance of task $i$ is represented by its success rate, $p_i(t) \in [0,1]$ at time $t$. The average performance of all tasks at time $t$ is described as below:
\begin{equation}
\mathrm{P}(t) := \frac{1}{N}\sum_{i=1}^{N}{p_i(t)}.
\end{equation}
\item \textbf{Forward Transfer.}
The forward transfer is measured by the normalized area between its training curve and the training curve of the single task performance. The $\mathrm{FT}$ is the average Forward Transfer at all tasks: 
\begin{equation}
\mathrm{FT}:=\frac{1}{N}\sum_{i=1}^{N}\frac{\frac{1}{\Delta}\int_{(i-1)\cdot\Delta}^{i\cdot\Delta}p_i(t)dt - \frac{1}{\Delta}\int_{(i-1)\cdot\Delta}^{i\cdot\Delta}p_i^b(t)dt}{1-\frac{1}{\Delta}\int_{(i-1)\cdot\Delta}^{i\cdot\Delta}p_i^b(t)dt},
\end{equation}
% \vskip -0.2in
% where the $\mathrm{AUC}_i:=\frac{1}{\Delta}\int_{(i-1)\cdot\Delta}^{i\cdot\Delta}p_i(t)dt$ and $\mathrm{AUC}_i^b:=\frac{1}{\Delta}\int_{(i-1)\cdot\Delta}^{i\cdot\Delta}p_i^b(t)dt$. 

\item \textbf{Catastrophic Forgetting.} For each task $i$, we measure the performance decrease after the whole training process for each tasks, by comparing with the performance of the end of task $i$.
\begin{equation}
\mathrm{CF} := \frac{1}{N}\sum_{i=1}^{N}{(p_i(i \cdot \Delta) - p_i(T))}.
\end{equation}
\end{itemize}

\newpage
\subsection{Ablation Study}
\input{content/ablation_study}

\section{Forward Transfer Results}\label{section:forward_transfer_results}
\begin{figure}[H]
\begin{center}
\centerline{\includegraphics[width=\linewidth]{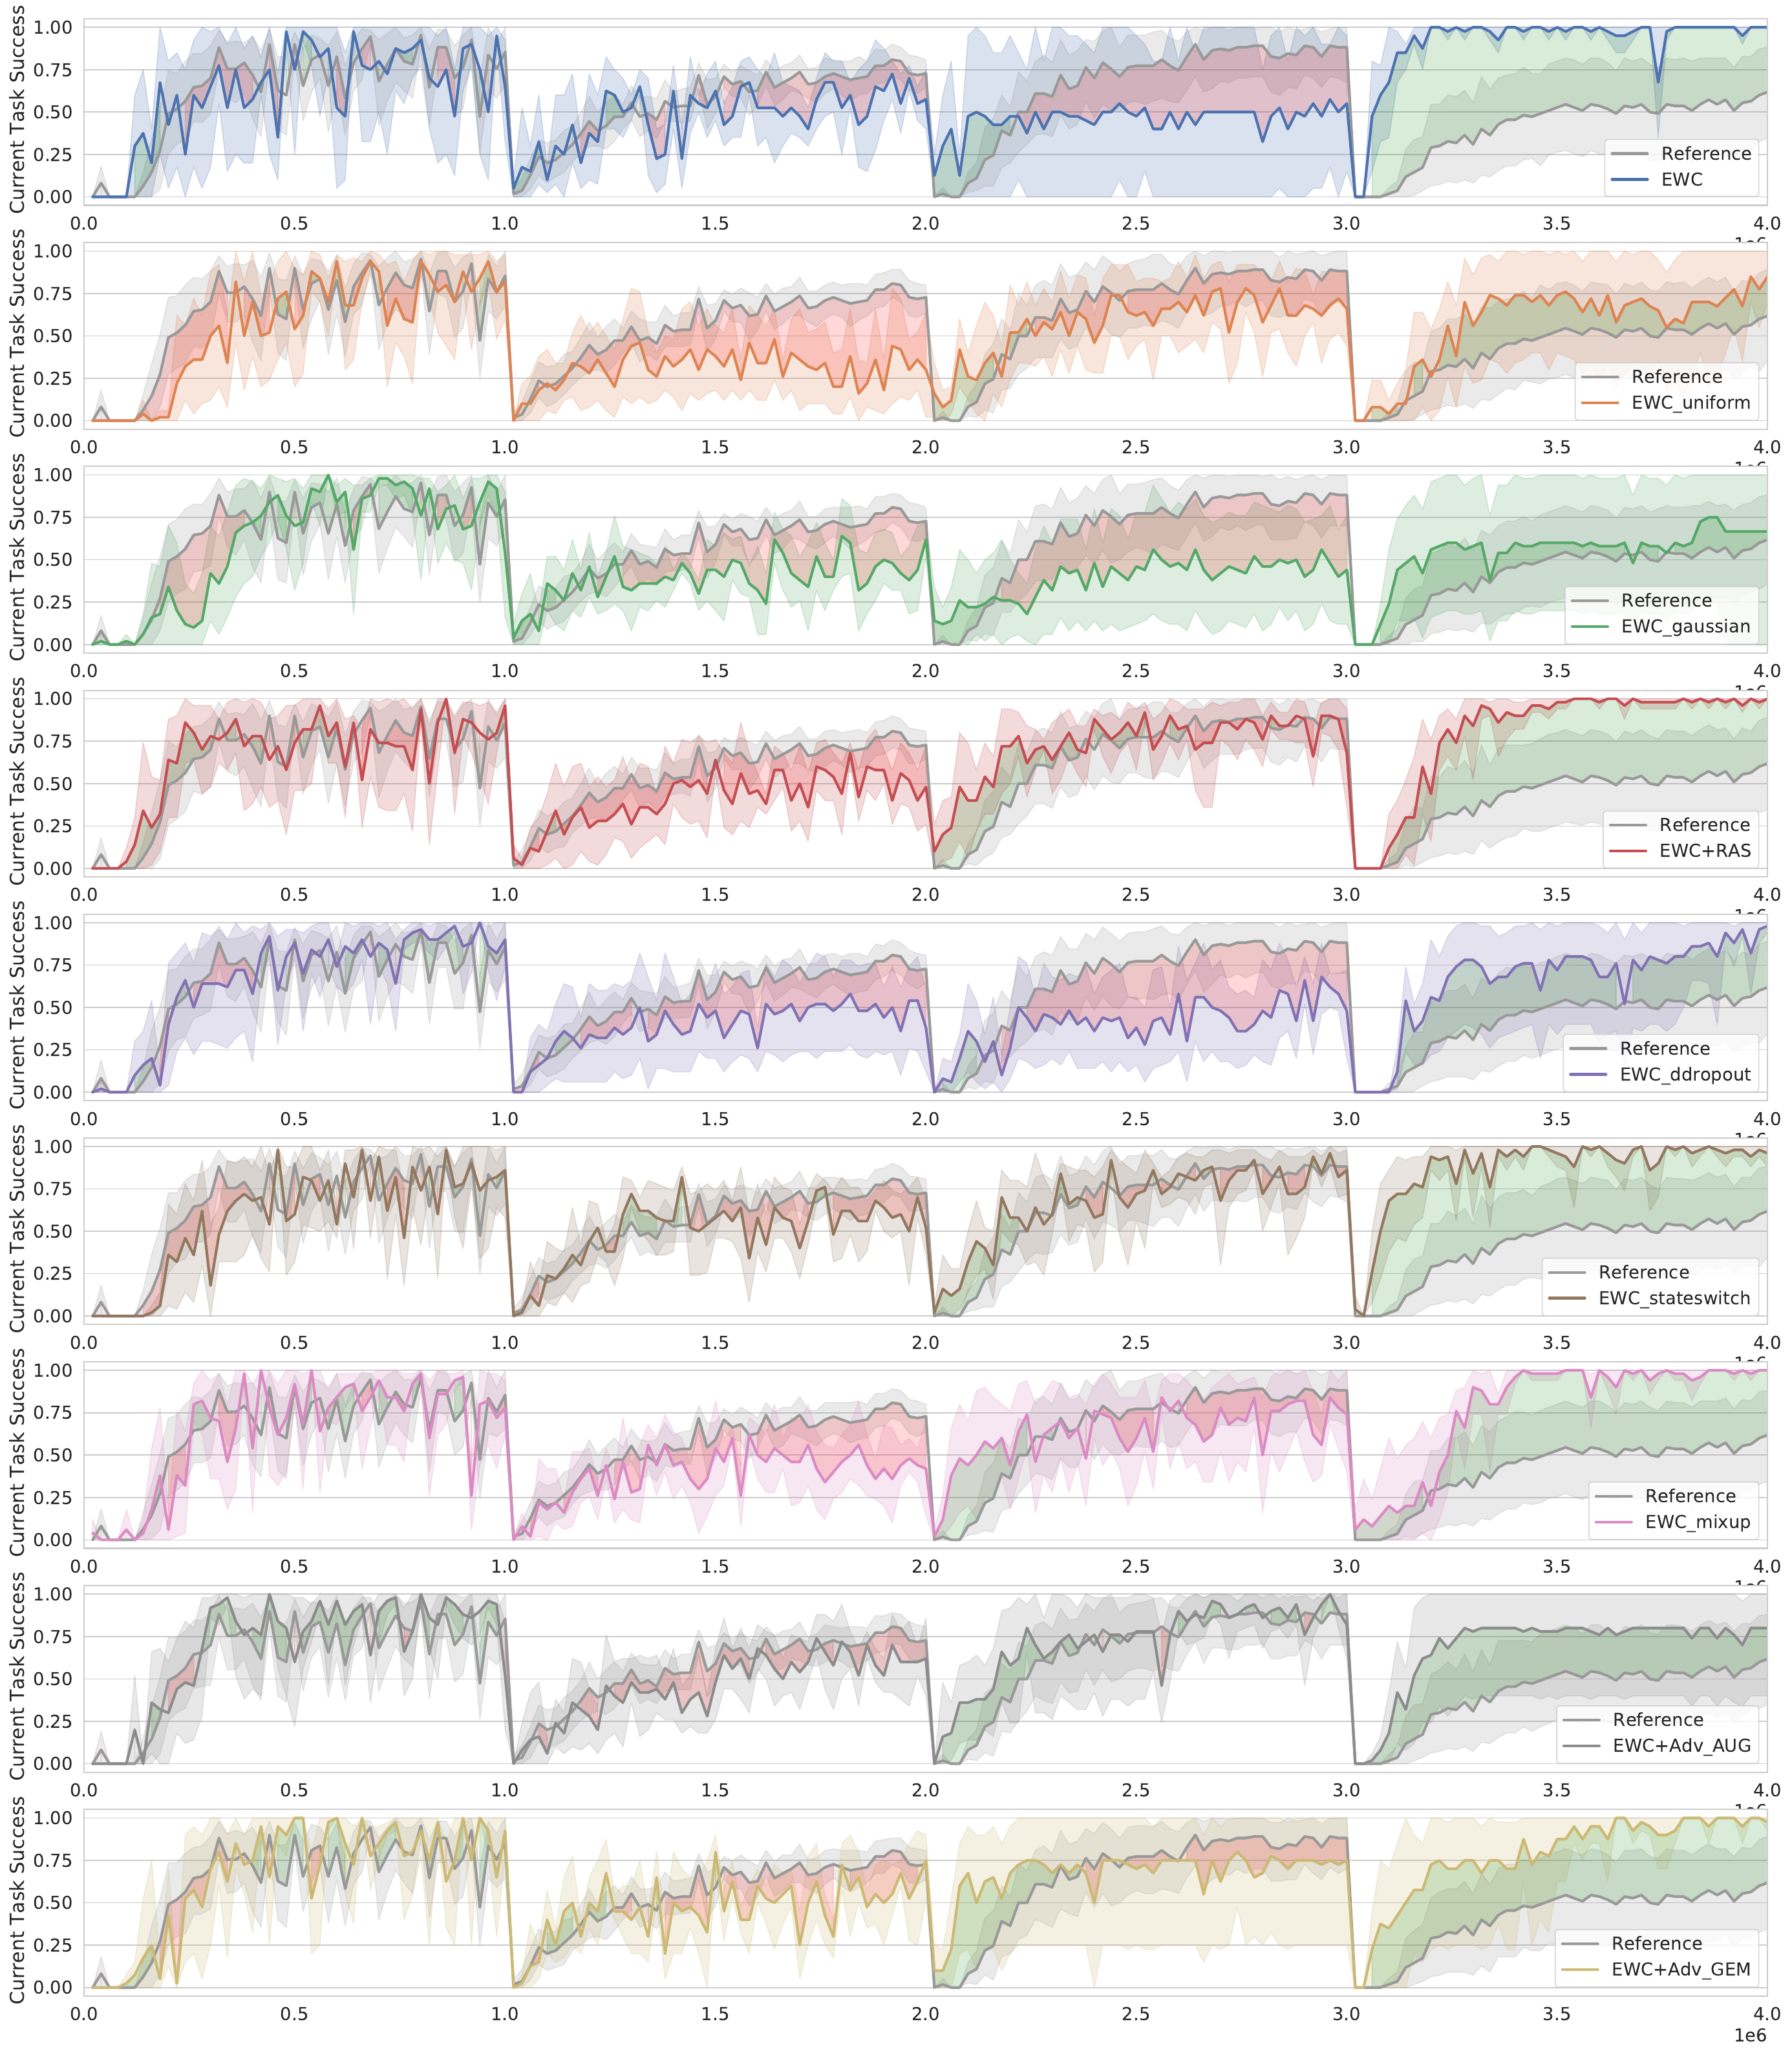}}
\caption{Forward Transfer for EWC method with different data augmentations. The reference curves come from the single-task training.}
\label{Figure:Apx_ForwardTransfer_EWC}
\end{center}
\end{figure}

\begin{figure}[ht]
\begin{center}
\centerline{\includegraphics[width=\linewidth]{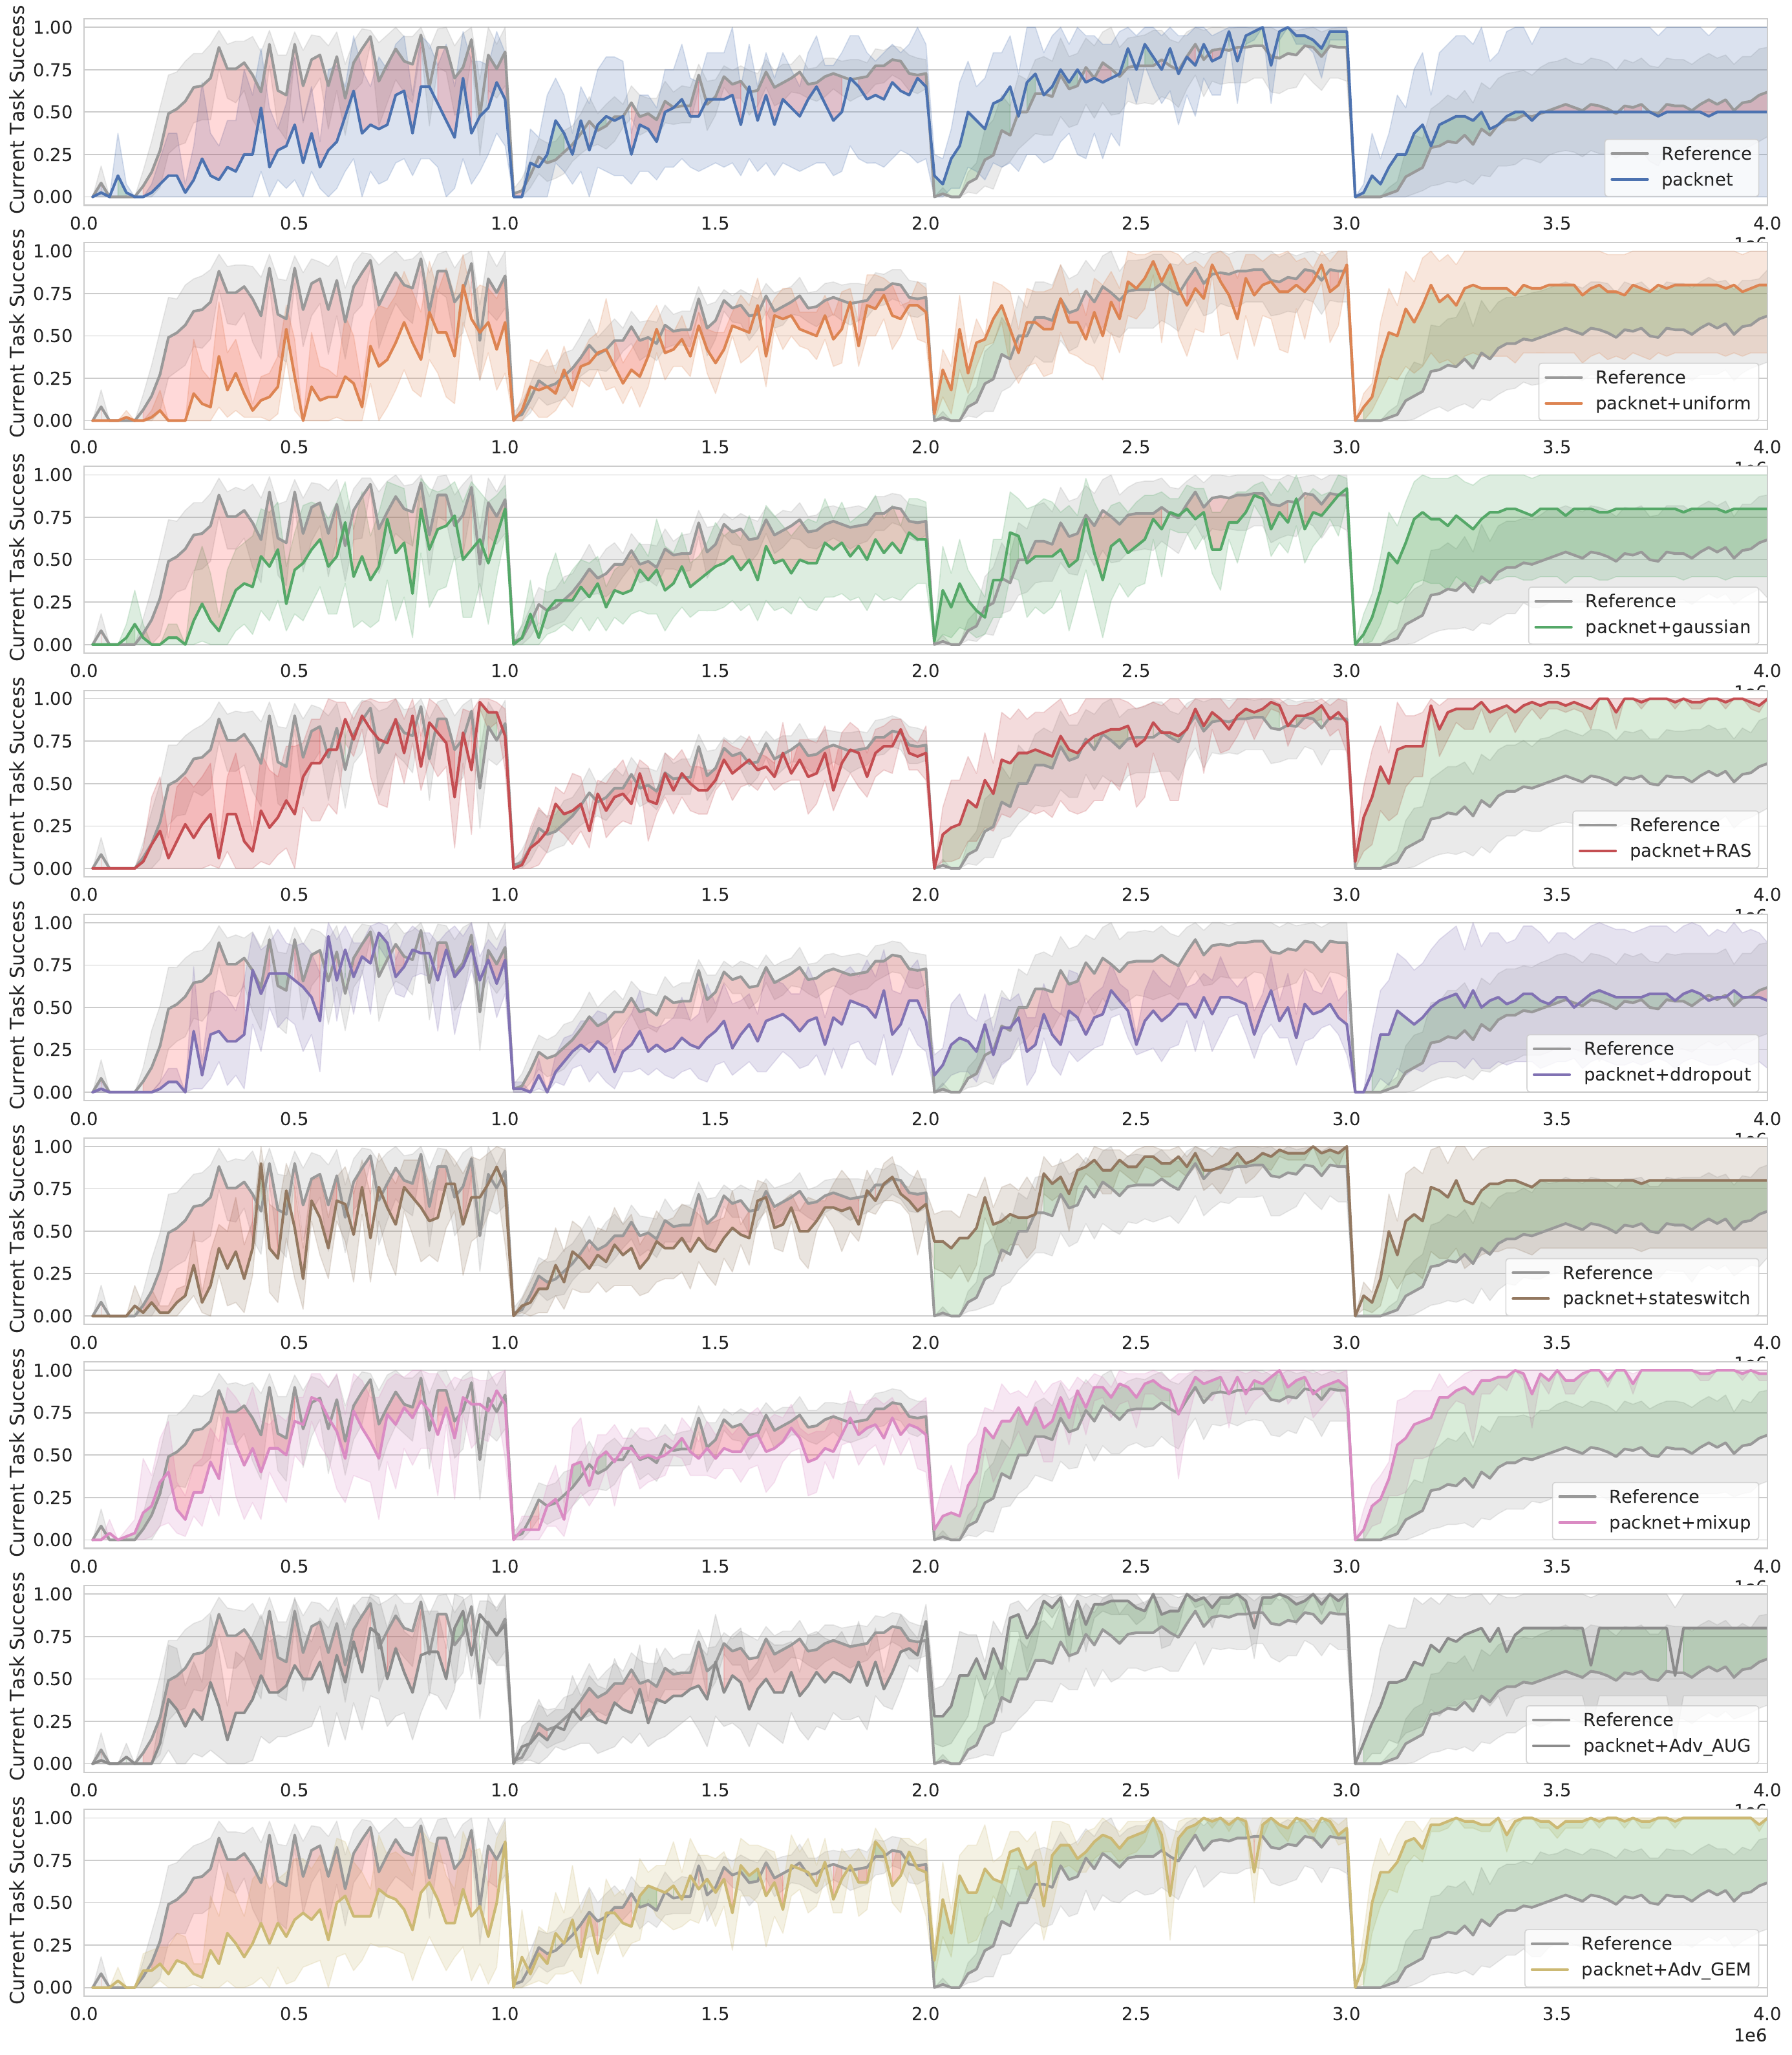}}
\caption{Forward Transfer for PackNet method with different data augmentations. The reference curves come from the single-task training.}
\label{Figure:ForwardTransfer_PackNet}
\end{center}
\end{figure}

% \begin{figure*}[htb] 
% \begin{center}
% \centerline{\includegraphics[width= \linewidth]{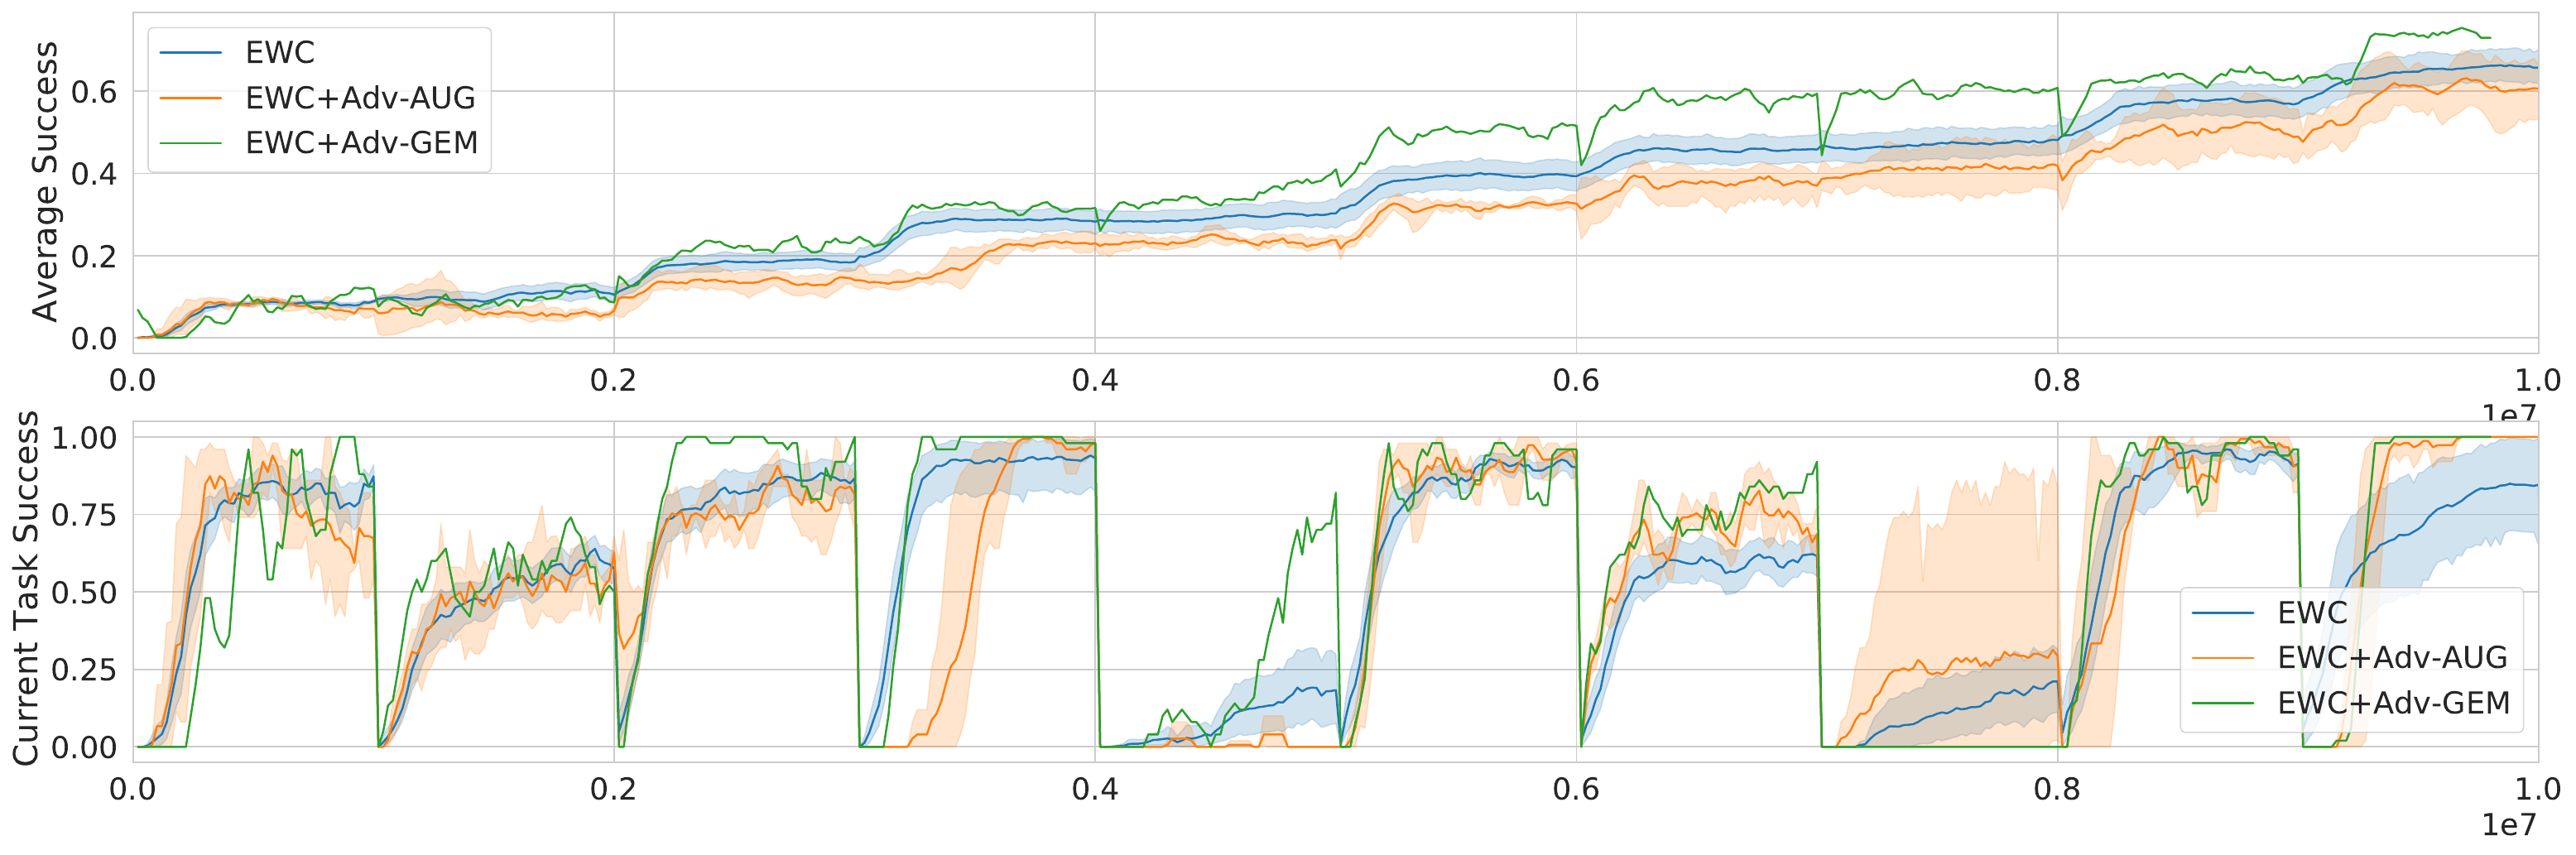}}
% \caption{Forward Transfer of \textit{PackNet}, \textit{PackNet + ras} and \textcolor{red}{PackNet + AD-AUG} in Test, 4 SEEDS, augmentation probability = 0.8}
% \label{figure:CW10}
% \end{center}
% \end{figure*}
